# Supplementary material for: Unstable Throughput: When the Difficulty Algorithm Breaks
Source: arXiv:2006.03044 source file (2021-04-30)
Supplement: Supplementary file 1 [file appendix.tex]

\appendix
\label{ref:appendix}

%%% ACF Plot of difficulty levels relative to 72 block moving avg. of difficulty
% \begin{figure}[hbpt]
% \centering
% \includegraphics[]{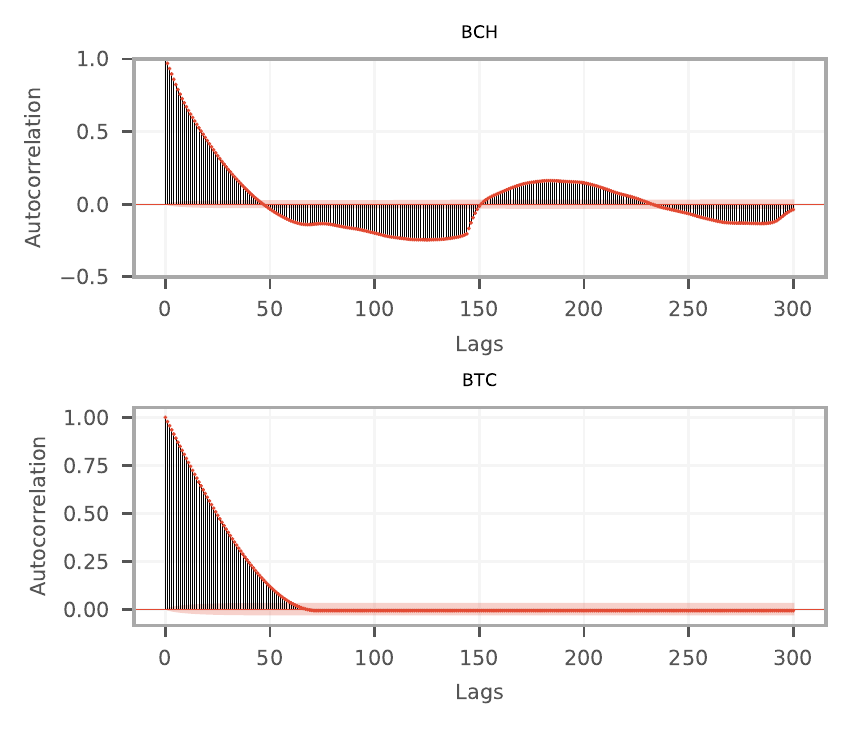}
% \caption{The autocorrelation of the block difficulty relative to the average difficulty of the past 72 blocks in BCH (top) and BTC (bottom) for the period 13 November, 2017 to 28 January, 2020.}
% \label{fig:acf_bch_btc}
% \end{figure}

%\section{Emergency Difficulty Algorithm}
%%% EDA block count BTC vs BCH

% \section{Variables and symbols}
% \label{app:variables}
% \begin{table}[htbp]
%   \label{tbl:sym}
%   \small
%   \renewcommand{\arraystretch}{1.2} 

%   \centering
    
%   \begin{tabular}{|c|p{47mm}|}
%     \hline
%     \textbf{Symbol} & \textbf{Description}\\
%     \hline
%     \hline
%     $D$ & Network difficulty\\
%     $D_i$ & Difficulty of block i\\
%     $T$ & Ideal inter block time\\
%     $\hat{H}$ & Estimated hash rate\\
%     $\hat{H}_i$ & Estimated hash rate for block i\\
%     $S$ & Decay/Smoothing factor\\
%     $t_i$ & Time of block i\\
%     $st_i$ & Solve time of block i\\
%     $T_A$ & Actual time elapsed between blocks\\
%     $W$ & Amount of work performed\\
%     $\overline{R}$ & Average rate of change in $D$\\
%     \hline
%   \end{tabular}
% \end{table}

\subsection{Emergency Difficulty Algorithm}\label{app:EDA}
When the BTC--BCH fork occurred on \nth{1} August 2017, BCH kept BTC's PoW puzzle, while slightly adapting its DA.
In BTC, the new difficulty $D^\prime$ is updated every $2\,016$ blocks based on the previous difficulty $D$, using the following formula:
\begin{align}
    D^\prime &= D \cdot \text{max}\left(\text{min}\left(\frac{2\,016 \cdot T}{T_A}, 4\right), \frac{1}{4}\right)
\end{align}
where $T$ is the ideal inter-block time and $T_A$ is the time it actually took to mine the last $2\,016$ blocks.

As miners could engage in coin-hopping strategies and the loyal hash rate was expected to be much lower than BTC's, BCH developers foresaw that a scenario such as the one described in the last paragraph of Section~\ref{sec:miner_incentives} would arise. 
To ensure stable block throughput during large effluxes of hash rate, BCH resorted to the \textit{Emergency Difficulty Algorithm} (EDA), whereby the difficulty would drop by $20$\% if the difference between $6$ successive block timestamps exceeded $12$ hours~\cite{aggarwal2019structural}.
Therefore, BCH's first DA was a combination of BTC's DA and the EDA.
However, it soon became apparent that this difficulty adjustment mechanism did not fulfill its objective.
Miners would stop mining BCH in order to cause consecutive $20$\% drops in the difficulty, which only adjusted back upwards every $2\,016$ blocks. 
Once the difficulty was sufficiently low, miners would switch back to mining BCH and produce many blocks at very low difficulty until the end of the $2\,016$ blocks window.
As a result of this miner behavior, from \nth{1} August 2017 to \nth{13} November 2017 a total of $9\,947$ more blocks were mined in BCH than in BTC (Figure~\ref{fig:eda_bch_btc} from Appendix~\ref{app:empirical}).

\subsection{Investigation: Coin-hopping Incentives}
Given the issues related to difficulty adjustments discussed in section~\ref{ref:background}, we empirically assess the extent to which miners are incentivized to engage in coin-hopping and therefore contribute towards the formation of the positive feedback loop.

\subsubsection{Deserts and Spikes}
For the purposes of this analysis we define a \textit{desert}, as a one hour interval during which at most $1$ block is mined
and a \textit{spike} as a one hour interval during which $12$ or more blocks are mined.
Note, we have chosen these thresholds s.t.\ their probabilities are small and relatively comparable.
Building on equation~\eqref{eq:blocksperhour}, we compute the probabilities of mining at most $k$ blocks per hour:
\begin{equation}
    P(K \leq k) = \sum\limits_{i = 0}^{k}P(K=i)
\end{equation}
Hence, we expect deserts and spikes to occur with a probability of $P(K \leq 1) = 1.74$\% and $1-P(K \leq 11) = 2.01$\%, respectively.
We refer to a period which is neither a spike nor a desert as a \textit{normal} period with $P(1 < K \leq 11) = 96.25$\%.

From Figure~\ref{fig:spikes_deserts} it becomes apparent that not only are the expected likelihoods of deserts and spikes not achieved, but that the situation appears to be aggravating over time.
For instance, over the last $6$ months of the examined period, deserts and spikes occurred $13.5$\% and $12.7$\% of the time, respectively.
By contrast, in BTC the respective percentages are $1.6$\% and $2.2$\%, which are significantly closer to the expected values.
\begin{figure}[H]
    \centering    \includegraphics{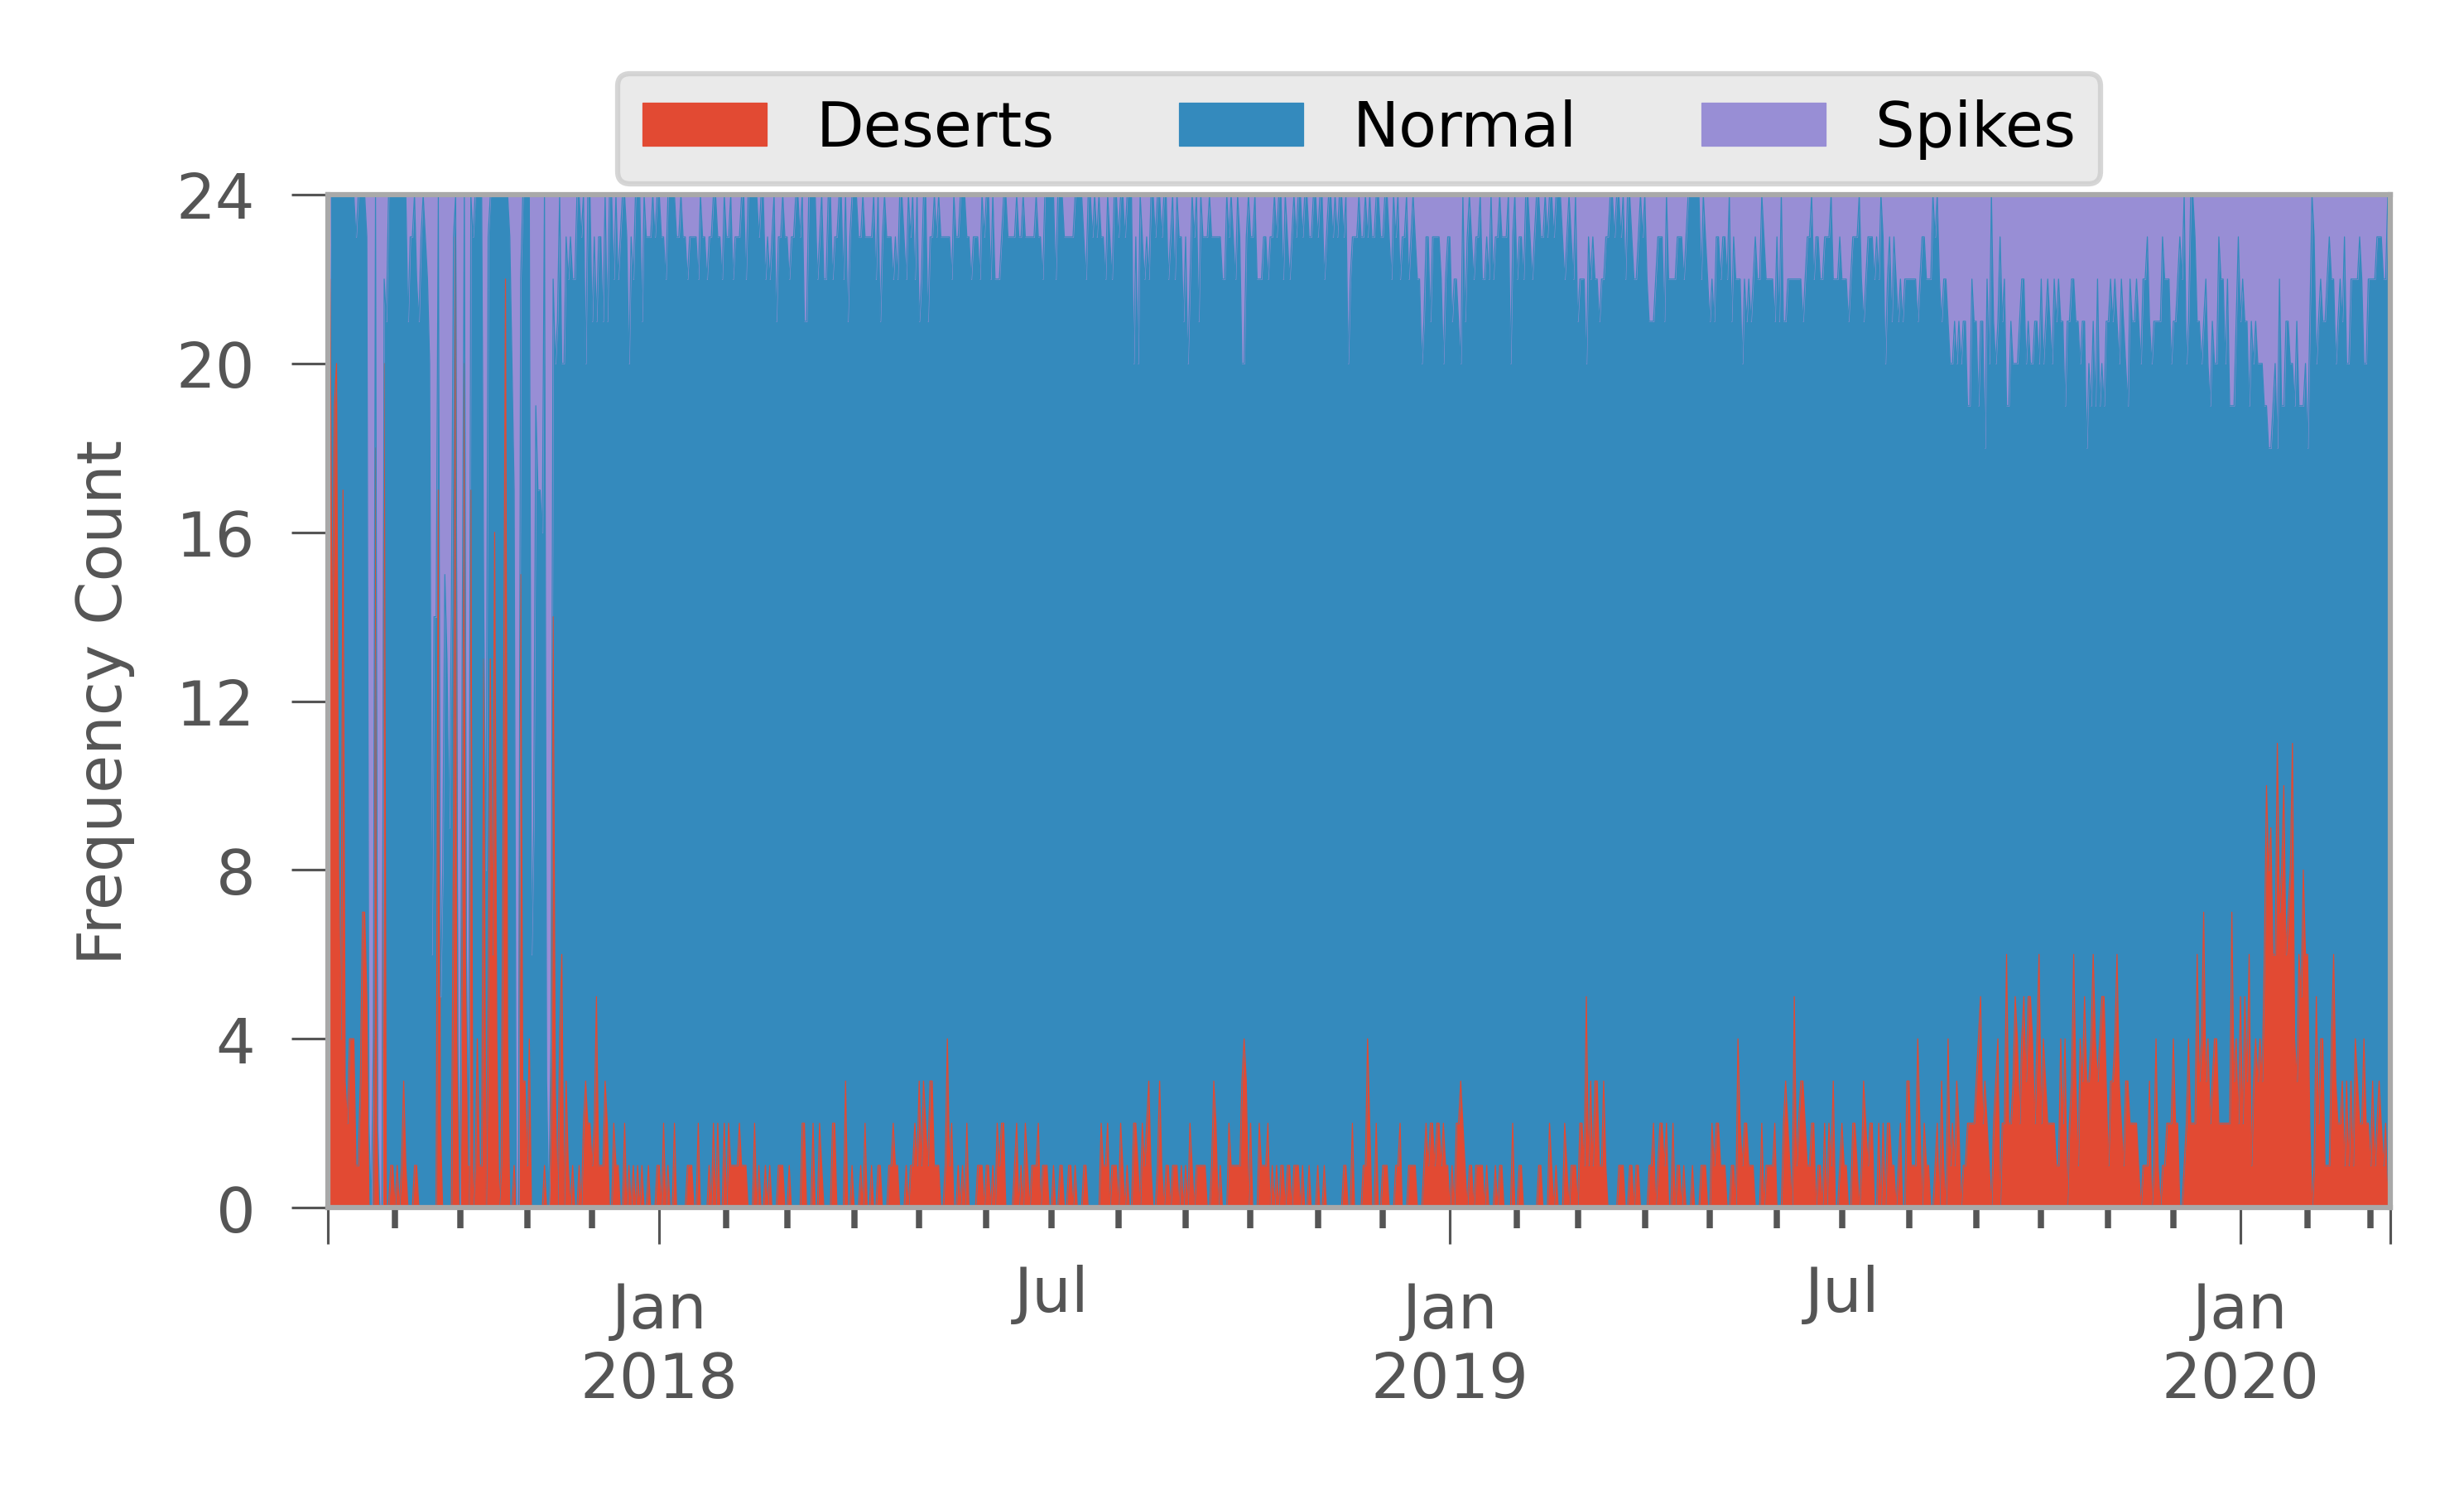}
    \caption{The number of one hour intervals classified as spikes, deserts, and normal periods in BCH.}
    \label{fig:spikes_deserts}
\end{figure}

\subsubsection{Mining Profitability Comparison}\label{sec:profitability}
We examine differences in the mining profitability of BCH and BTC by comparing the ratio of their DARIs (i.e.\ BCH DARI over BTC DARI) in Figure~\ref{fig:dari_ratio}.
In the long term, mining either coin is equally profitable as the average DARI ratio has a value of $1.0266$.
However, as the ratio frequently oscillates this incentivizes miners to adopt a coin-hopping strategy. 
Notably, in the latter months, the oscillations become significantly more frequent and consistently reaching deviations of 10\% and even 15\% either in favor of BCH or BTC. 
These fluctuations are reflected in an increased number of spikes and deserts during the same period as can be seen in Figure~\ref{fig:spikes_deserts}.

\begin{figure}[H]
    \centering
    \includegraphics[width=0.47\textwidth]{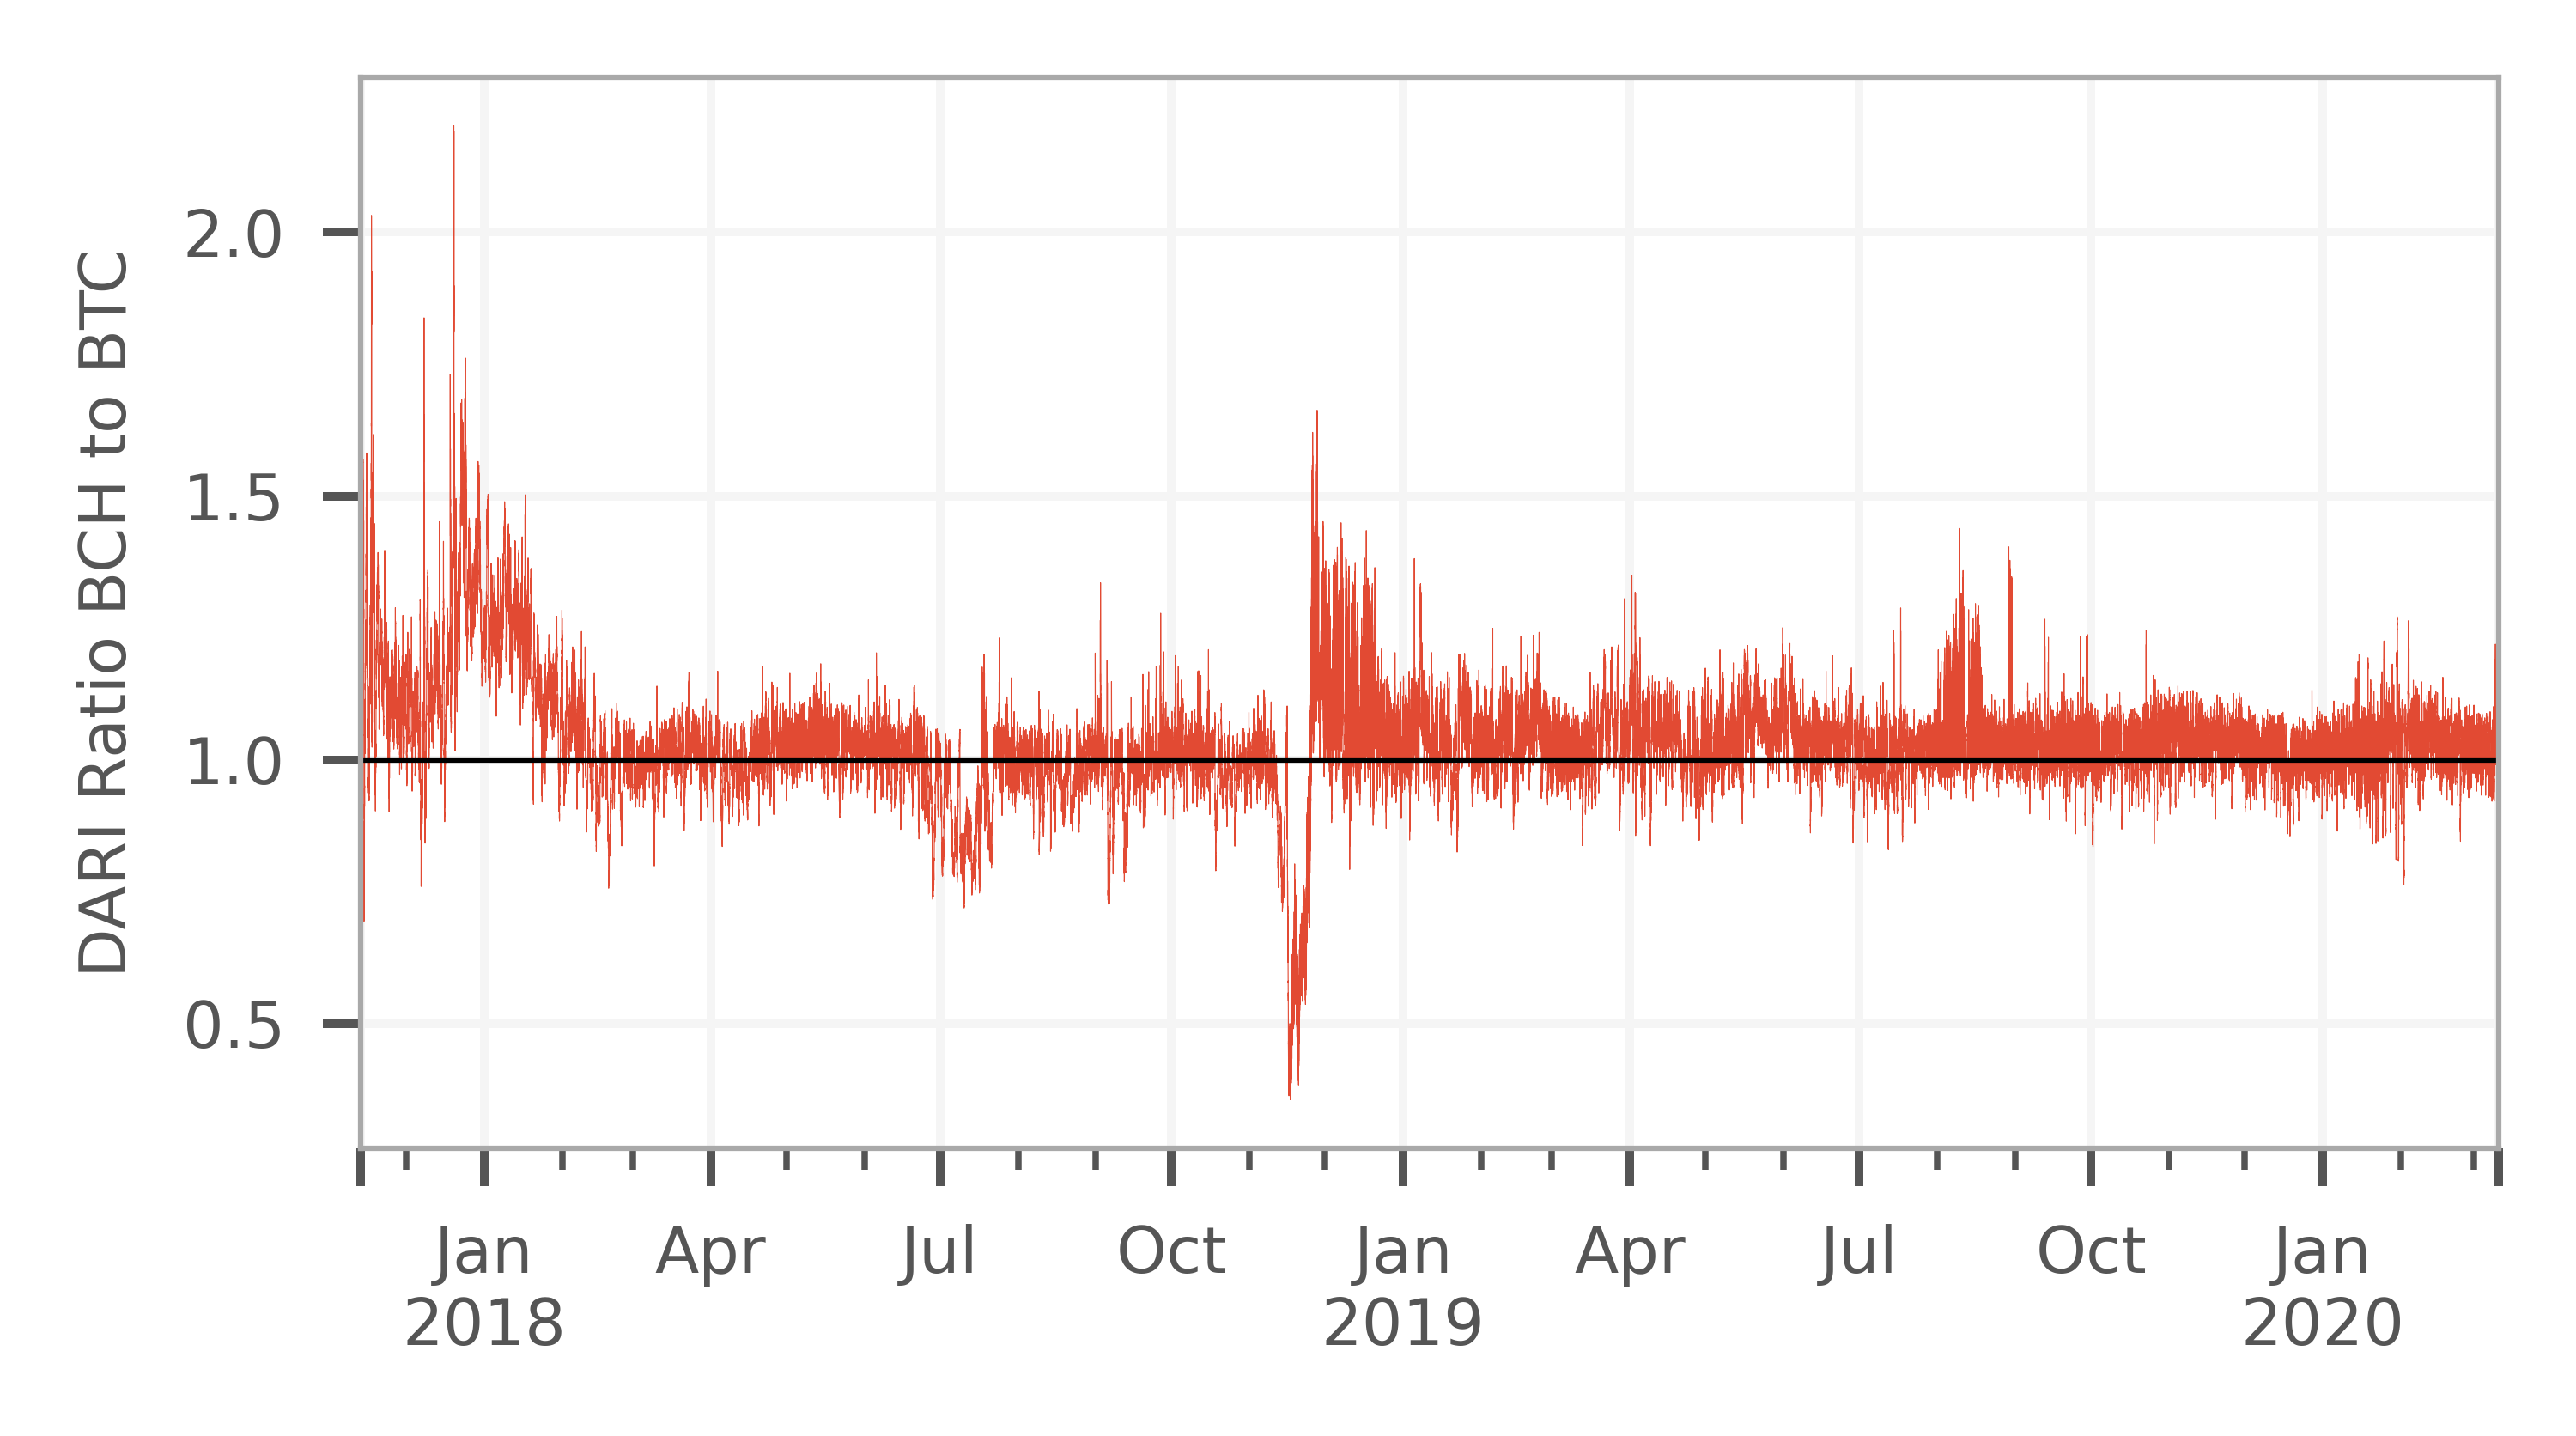}
    \caption{The minute average DARI ratio of BCH to BTC. Equal profitability is shown by the black line.}
    \label{fig:dari_ratio}
\end{figure}

\subsubsection{Miner Analysis}\label{sec:miner-analysis}
In order to examine the extent to which miners benefit from mining BCH, we analyze the block distribution for a set of high hash rate miners between \nth{11} September 2019 and \nth{11} March 2020.
We deem this period relevant as the number of spikes and deserts is considerably higher than before.

In Table~\ref{tab:bch_miners}, we give data for the five largest BCH mining pools\footnote{A mining pool allows multiple miners to combine their computational efforts and share the rewards. A pool can be seen as a single miner entity.} (BTC.TOP, Antpool, BTC.com, ViaBTC, Huobi Pool) and three large miners without known identities, sorted by their respective shares of total blocks mined during the examined period.
\begin{table}[H]
  \centering
  \begin{tabular}{l|llll}
    {} & \multicolumn{4}{c}{\textbf{\% of Total Blocks Mined in:}}\\
    \thead[l]{Miner} & \thead[l]{Normal} & \thead[c]{Spikes} & \thead[r]{Deserts} & \thead[l]{Total}\\ %\thead[l]{Avg. Work \\per Block\\ (GH)}\\
    \toprule
    % Pools
    BTC.TOP & $8.95$ & $8.28$ & $0.12$ & $17.35$\\% & 441.12\\
    Antpool & $8.40$ & $1.84$ & $0.29$ & $10.53$\\% & 478.77\\
    \texttt{qp4ajq\dots} & $2.36$ & $6.76$ & $0.00$ & $9.12$\\% 483.15\\
    BTC.com & $6.80$ & $1.18$ & $0.31$ & $8.29$\\% & 436.96\\
    \texttt{qqq9v3\dots} & $2.21$ & $5.36$ & $0.00$ & $7.57$\\% 334.50\\
    ViaBTC & $5.91$ & $1.18$ & $0.29$ & $7.38$\\% & 450.05\\
    \texttt{qzkuv6\dots} & $2.77$ & $2.39$ & $0.00$ & $5.16$\\% 360.39\\
    Huobi Pool & $2.47$ & $0.73$ & $0.06$ & $3.26$\\
    % \midrule
    % \texttt{qqn4z4\dots} & 3.86 & 0.87 & 0.10 & 4.83\\% 389.36\\
    % \texttt{ppmwv6\dots} & 3.53 & 0.66 & 0.06 & 4.25\\% 377.45\\
    % \texttt{ppwq0p\dots} & 3.39 & 0.58 & 0.15 & 4.12\\% 369.54\\
    % \midrule
    % Others & 13.03 & 4.87 & 0.23 & 18.13\\% & 460.40\\
    \bottomrule
  \end{tabular}
  \caption{Proportion of blocks mined by large miners during normal, spike and desert periods between block numbers 599798 and 625989.}
  \label{tab:bch_miners}
\end{table}

Interestingly, out of the five largest mining pools, only BTC.TOP mined a similar amount of blocks during spikes and normal periods, while the remaining four pools mined on average 4.66\% less blocks during spikes.
This indicates that BTC.TOP is the only pool that successfully engages in coin-hopping by mining with higher hash rate during periods of lower difficulty.
The other pools lose part of their block share to the coin-hopping miners.
For instance, miners \texttt{qp4ajq} and \texttt{qqq9v3} obtained the third and fifth highest shares of blocks, while mining more than $70$\% of their blocks during spikes\footnote{Full address of miners from Table~\ref{tab:bch_miners} are given in Table~\ref{tab:bch_addresses} from Appendix~\ref{app:empirical}.} and, perhaps rather impressively, none during deserts.

The extent of such coin-hopping behavior can also be measured by analyzing the fluctuation in BCH's hash rate. 
The logarithmic scale chart from Figure~\ref{fig:hashrate_btc_bch} shows the hash rates of BTC and BCH over the last 6 months, estimated using a moving average of $6$ blocks.
While BTC's hash rate consistently oscillates from approx.\ $90$ to $180$ Exahashes per second, BCH's hash rate fluctuates from approx.\ $2$ to $18$ Exahashes per second.
This means that BCH experiences periods when the hash rate increases even $9$ times relatively to the baseline hash rate, which is inline with the results of Table~\ref{tab:bch_miners}.
\begin{figure}[H]
    \centering
    \includegraphics[width=0.47\textwidth]{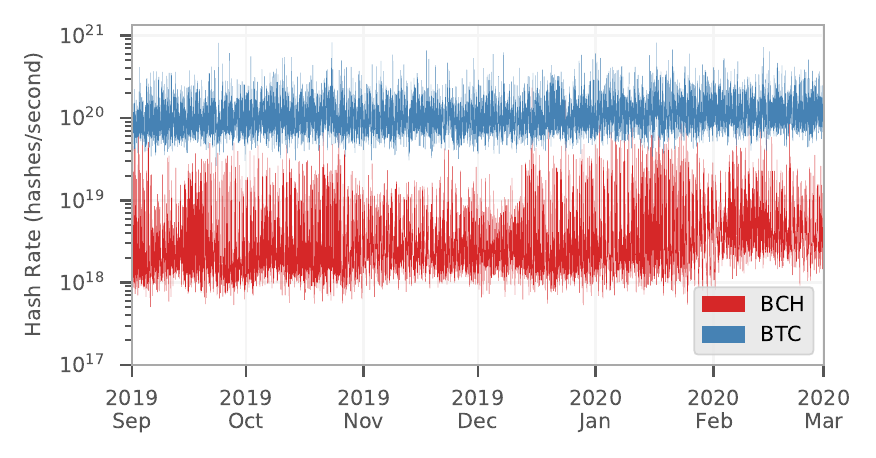}
    \caption{Estimated hash rates of BTC and BCH using a 6 block average.}
    \label{fig:hashrate_btc_bch}
\end{figure}

\section{Additional Figures}
\label{app:empirical}
\label{app:simulations}
\label{app:model}

\begin{figure}[H]
\centering
\includegraphics[width=0.47\textwidth]{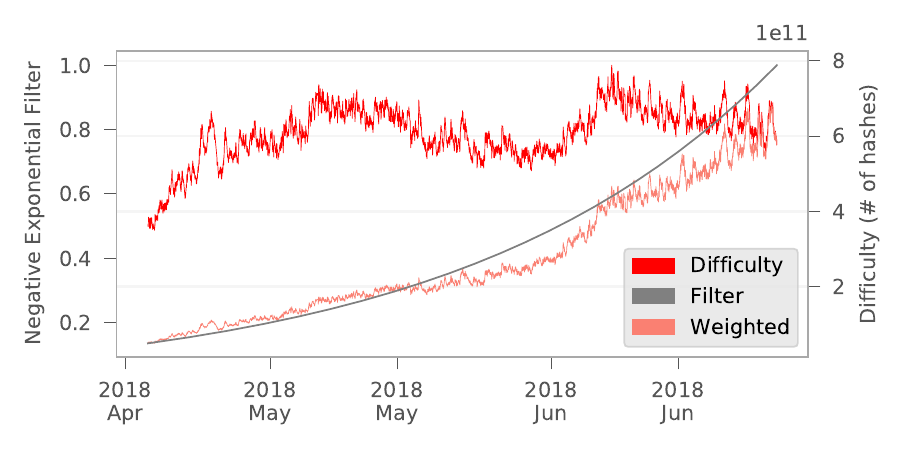}
\caption{Difficulties of 10\,000 blocks are filtered with a negative exponential to obtain the weighted difficulties.}
\label{fig:diff_exp_filter_blocks}
\end{figure}

\begin{figure}[H]
\centering
\includegraphics[]{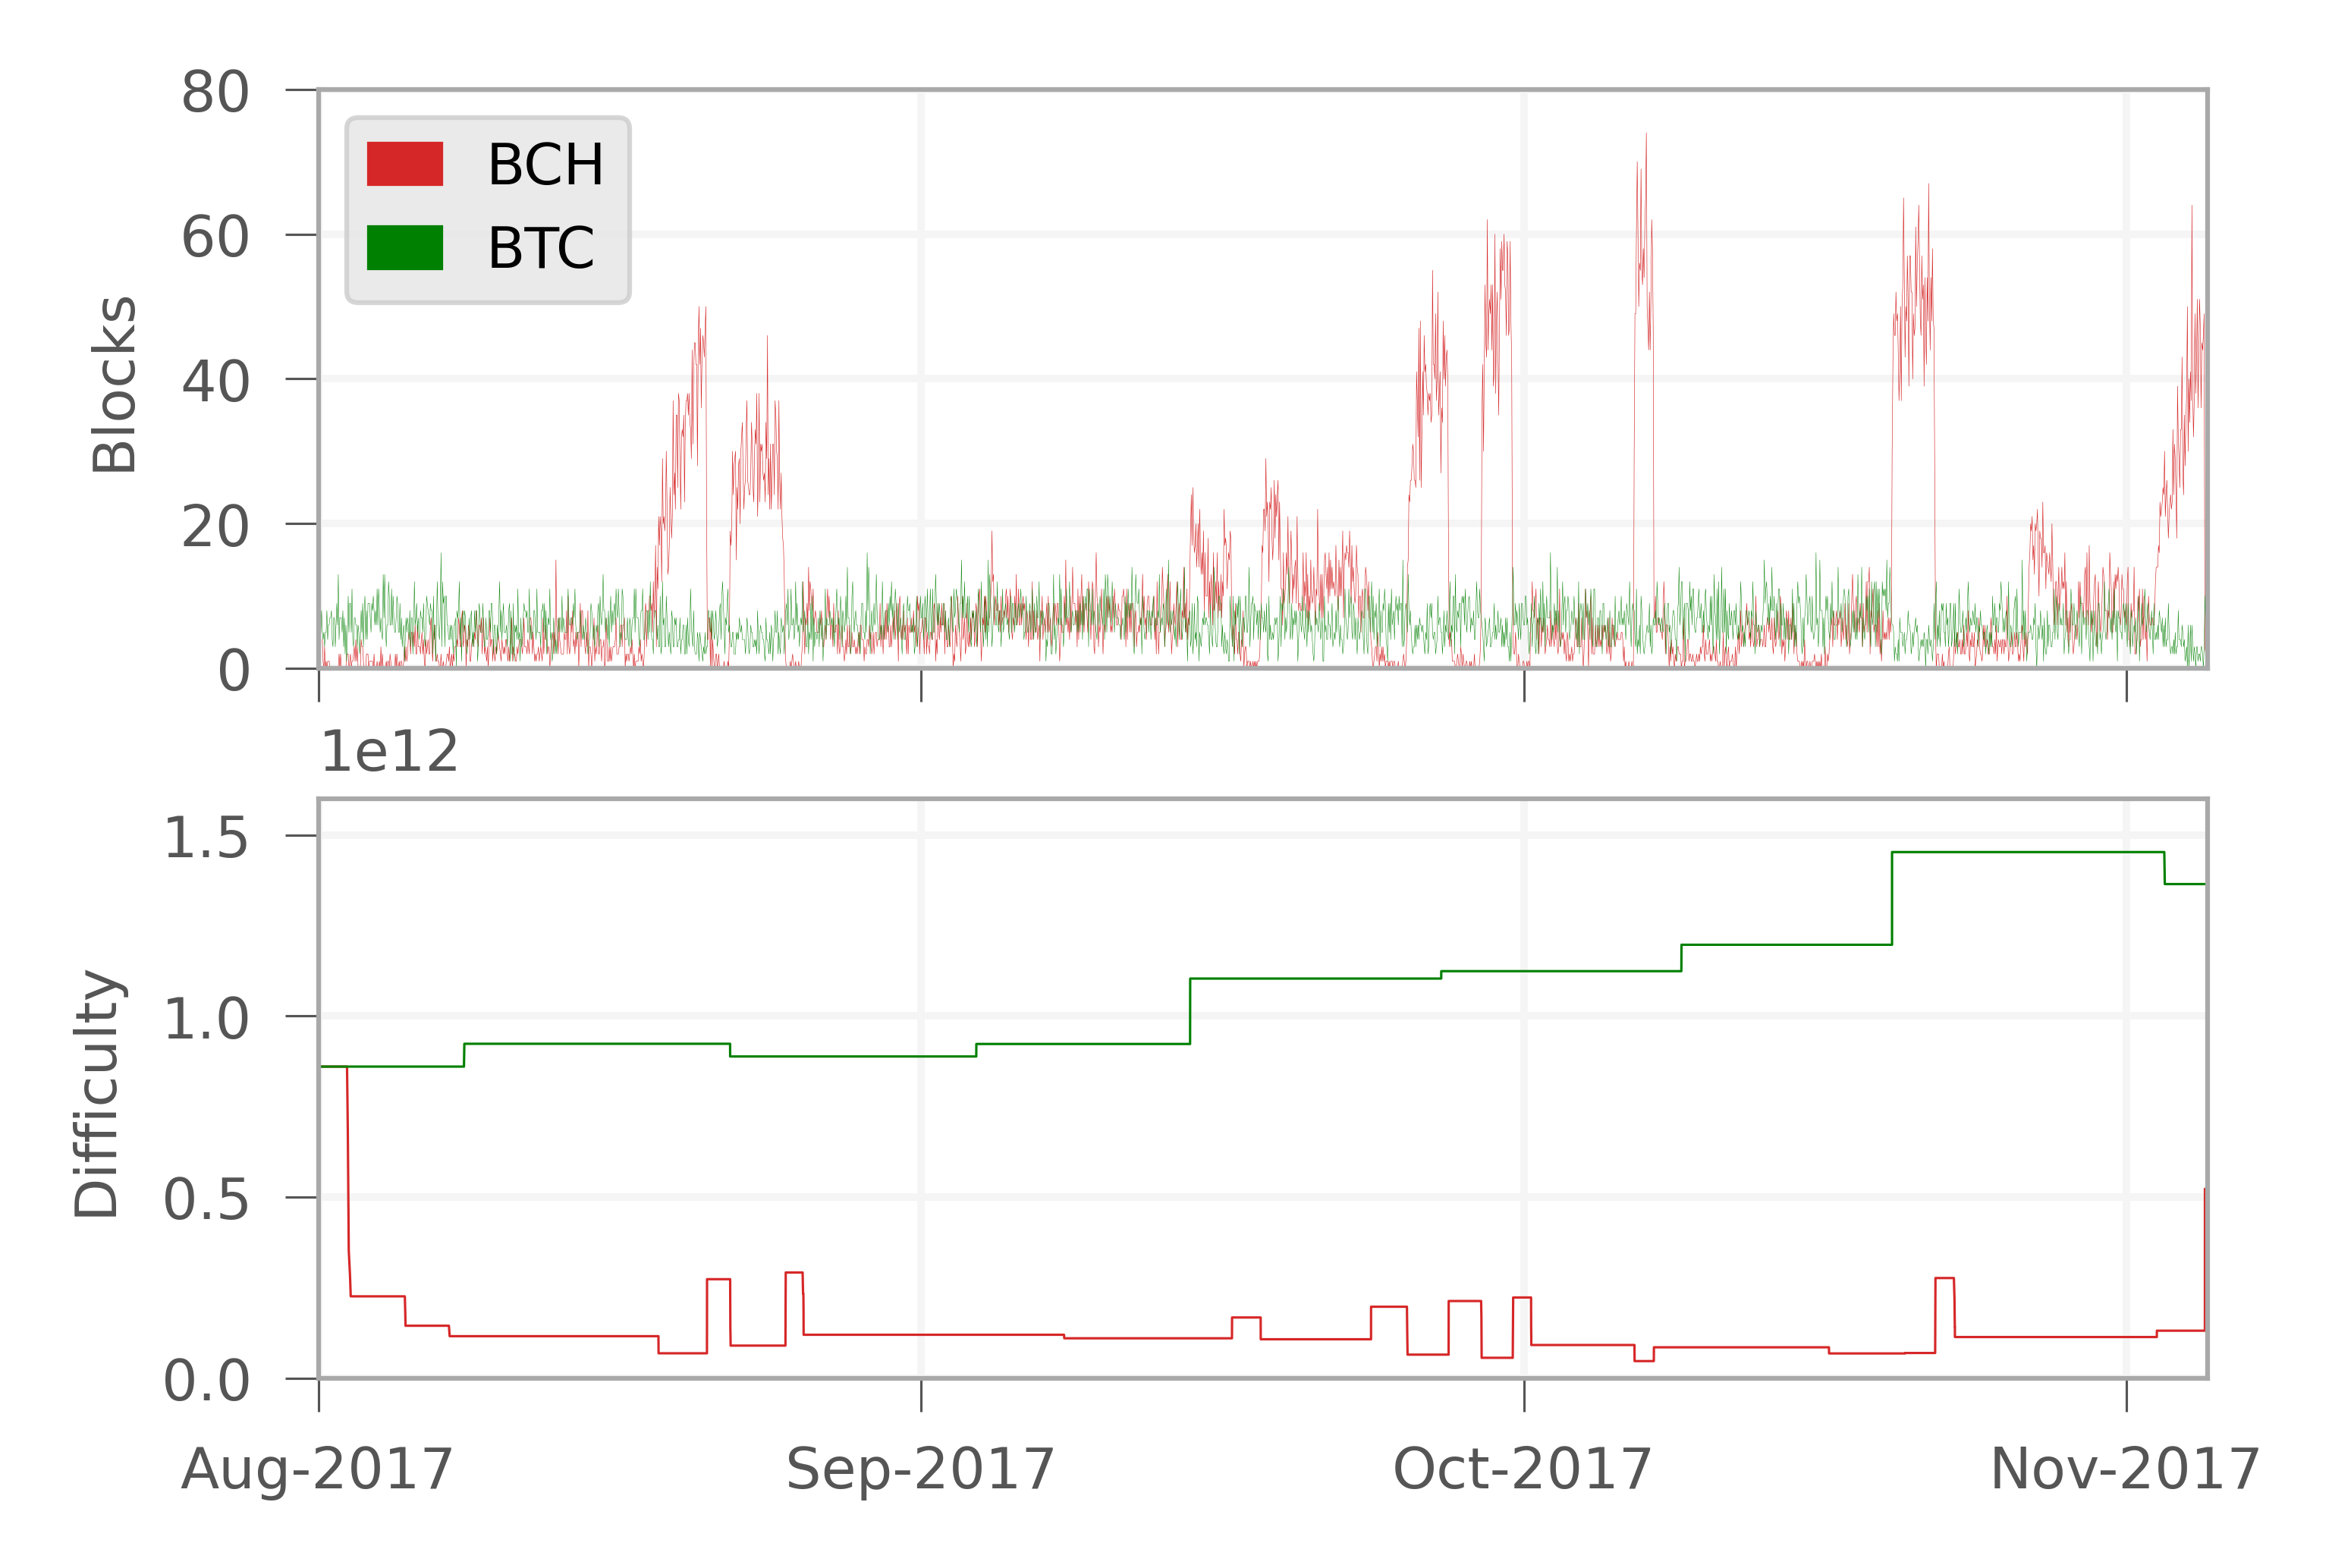}
\caption{Number of blocks mined per hour (top) and block difficulties (bottom) for the period during which the Emergency Difficulty Algorithm was active.}
\label{fig:eda_bch_btc}
\end{figure}

\begin{figure}[H]
\centering
\includegraphics[trim={0 0.95cm 0 0},clip,width=0.48\textwidth]{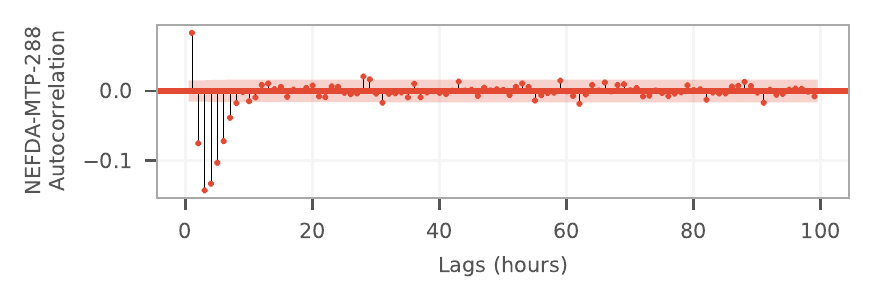}
\includegraphics[trim={0 0.95cm 0 0},clip,width=0.48\textwidth]{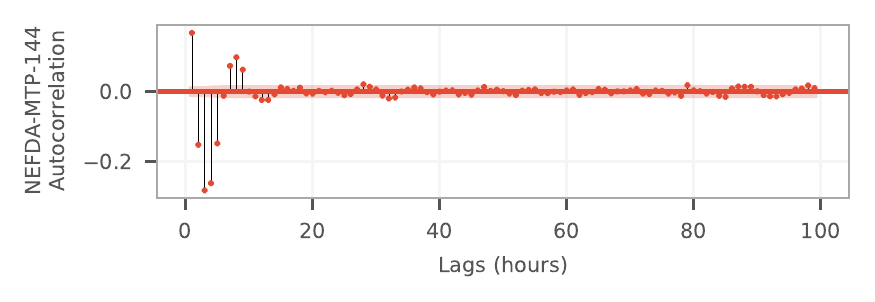}
\includegraphics[trim={0 0.95cm 0 0},clip,width=0.48\textwidth]{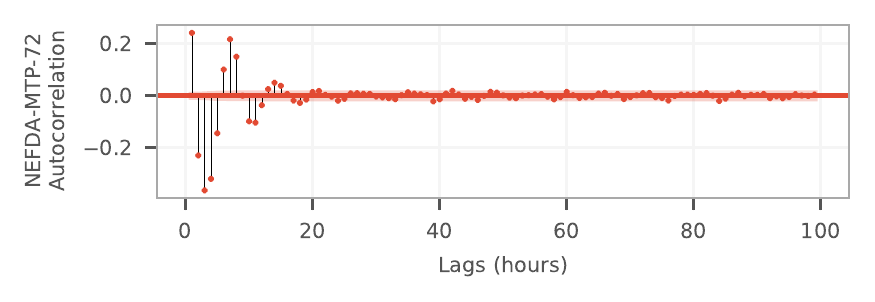}
\includegraphics[trim={0 0.95cm 0 0},clip,width=0.48\textwidth]{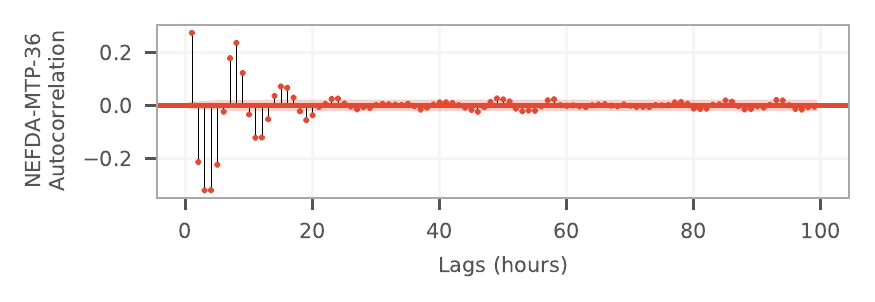}
\includegraphics[width=0.48\textwidth]{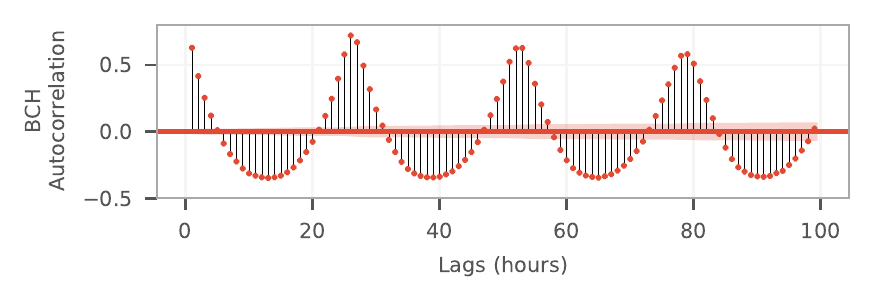}

\caption{The autocorrelation in number of blocks mined per hour for NEFDA--MTP with smoothing factors 288, 144, 72 and 36, as well as for BCH in a coin hopping simulation of 100\,000 blocks.}
\label{sim:smoothing-acfs-summary}
\end{figure}

\begin{footnotesize}
\begin{table}[H]
  \centering
  \begin{tabular}{ll}
    %\toprule
    \thead[l]{Address} & \thead[l]{Miner}\\
    \toprule    
    qpk4hk3wuxe2uqtqc97n8atzrrr6r5mleczf9sur4h & BTC.TOP\\
    qqfc3lxxylme0w87c5j2wdmsqln6e844xcmsdssvzy & Antpool\\
    qrcuqadqrzp2uztjl9wn5sthepkg22majyxw4gmv6p & ViaBTC\\
    qrd9khmeg4nqag3h5gzu8vjt537pm7le85lcauzezc & BTC.com\\
    qrjc9yecwkldlhzys3euqz68f78s2wjxw5h6j9rqpq & Huobi Pool\\
    qp4ajqctqvx5m5fhpswdkgm9whwsapgst5twl9zd5h & unknown\\ 
    qqq9v3hhl0vga8w5cts6dx5aa8xep2v2ssvppp5xcn & unknown\\
    qzkuv6ftvt28v6hauv44r58tjupsgn3nqsnslfxzqf & unknown\\ 
    % \texttt{qqn4z4d3g5kc044munahy2wt05uek333lgwszmxgzw} & unknown\\
    % \texttt{ppmwv6dexxhsjkw0xurt6jcsrl5desswpc6zgzy9f7} & unknown\\
    % \texttt{ppwq0ptyt2lnq2yd7hrttr00qacmxznuzqcncmhd49} & unknown\\
    \bottomrule
  \end{tabular}
  \caption{The Bitcoin Cash addresses for selected miners.}
  \label{tab:bch_addresses}
\end{table}
\end{footnotesize}

\begin{figure}[H]
\centering
\includegraphics[width=0.48\textwidth]{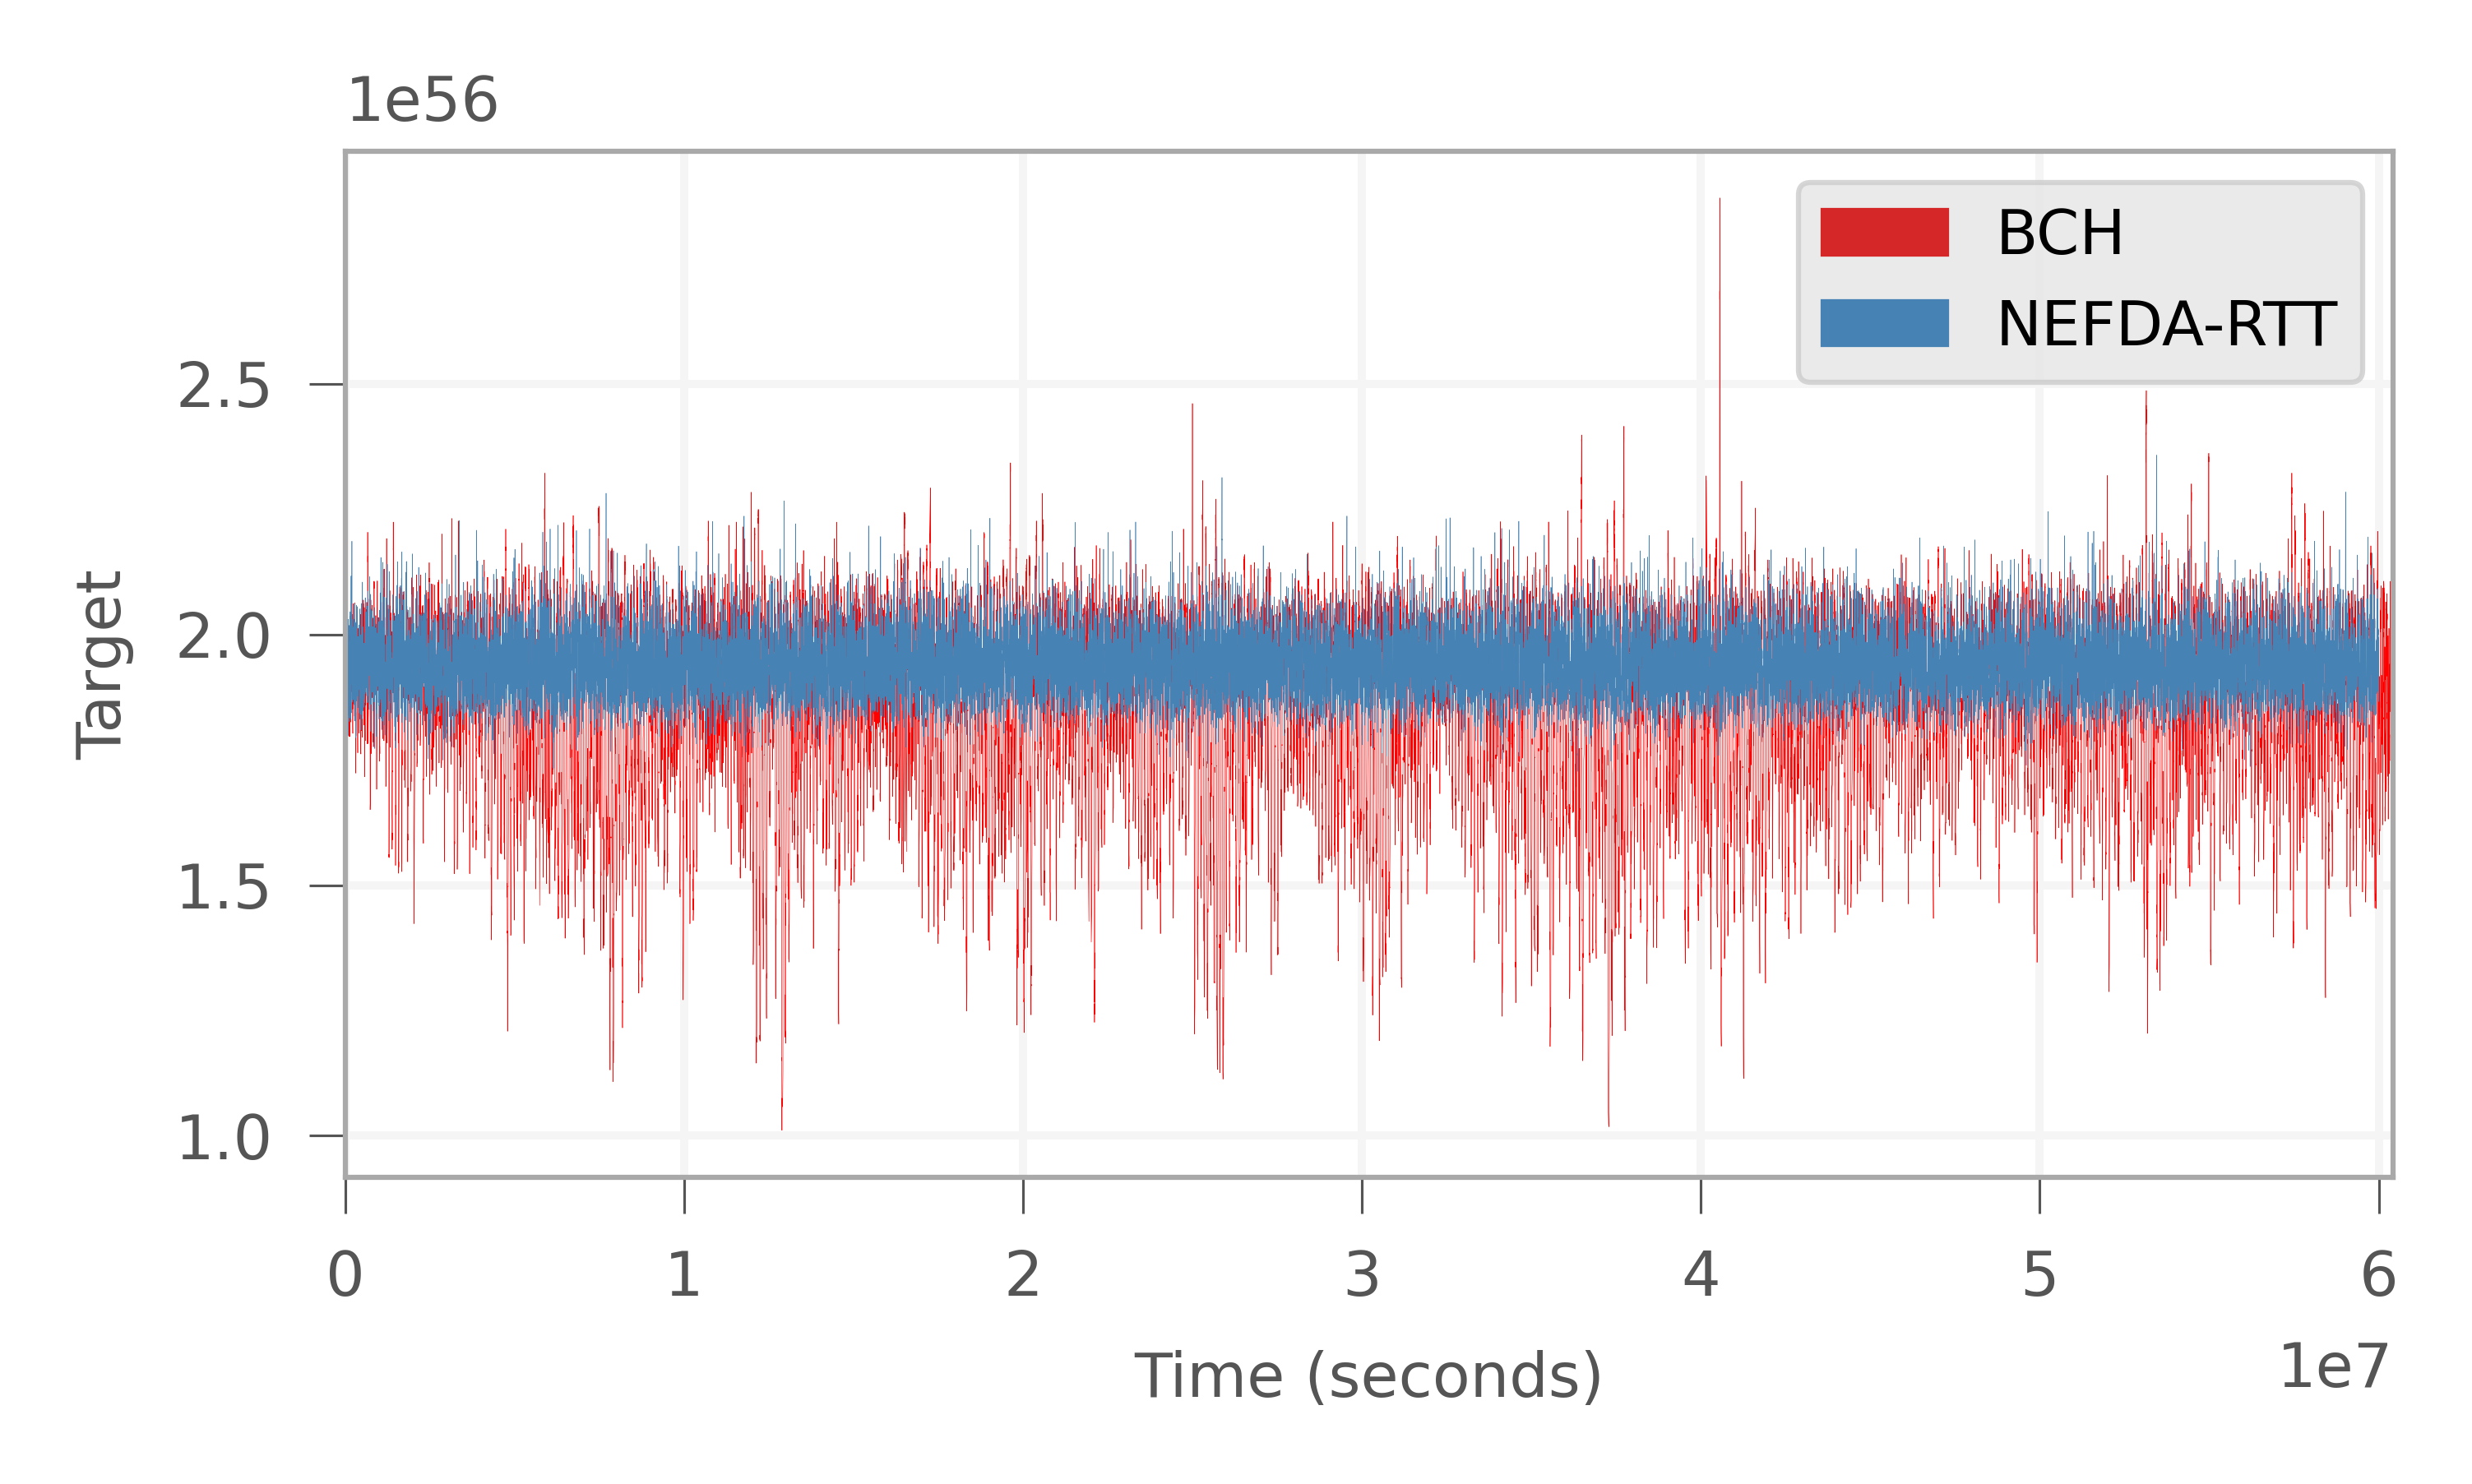}
\includegraphics[width=0.48\textwidth]{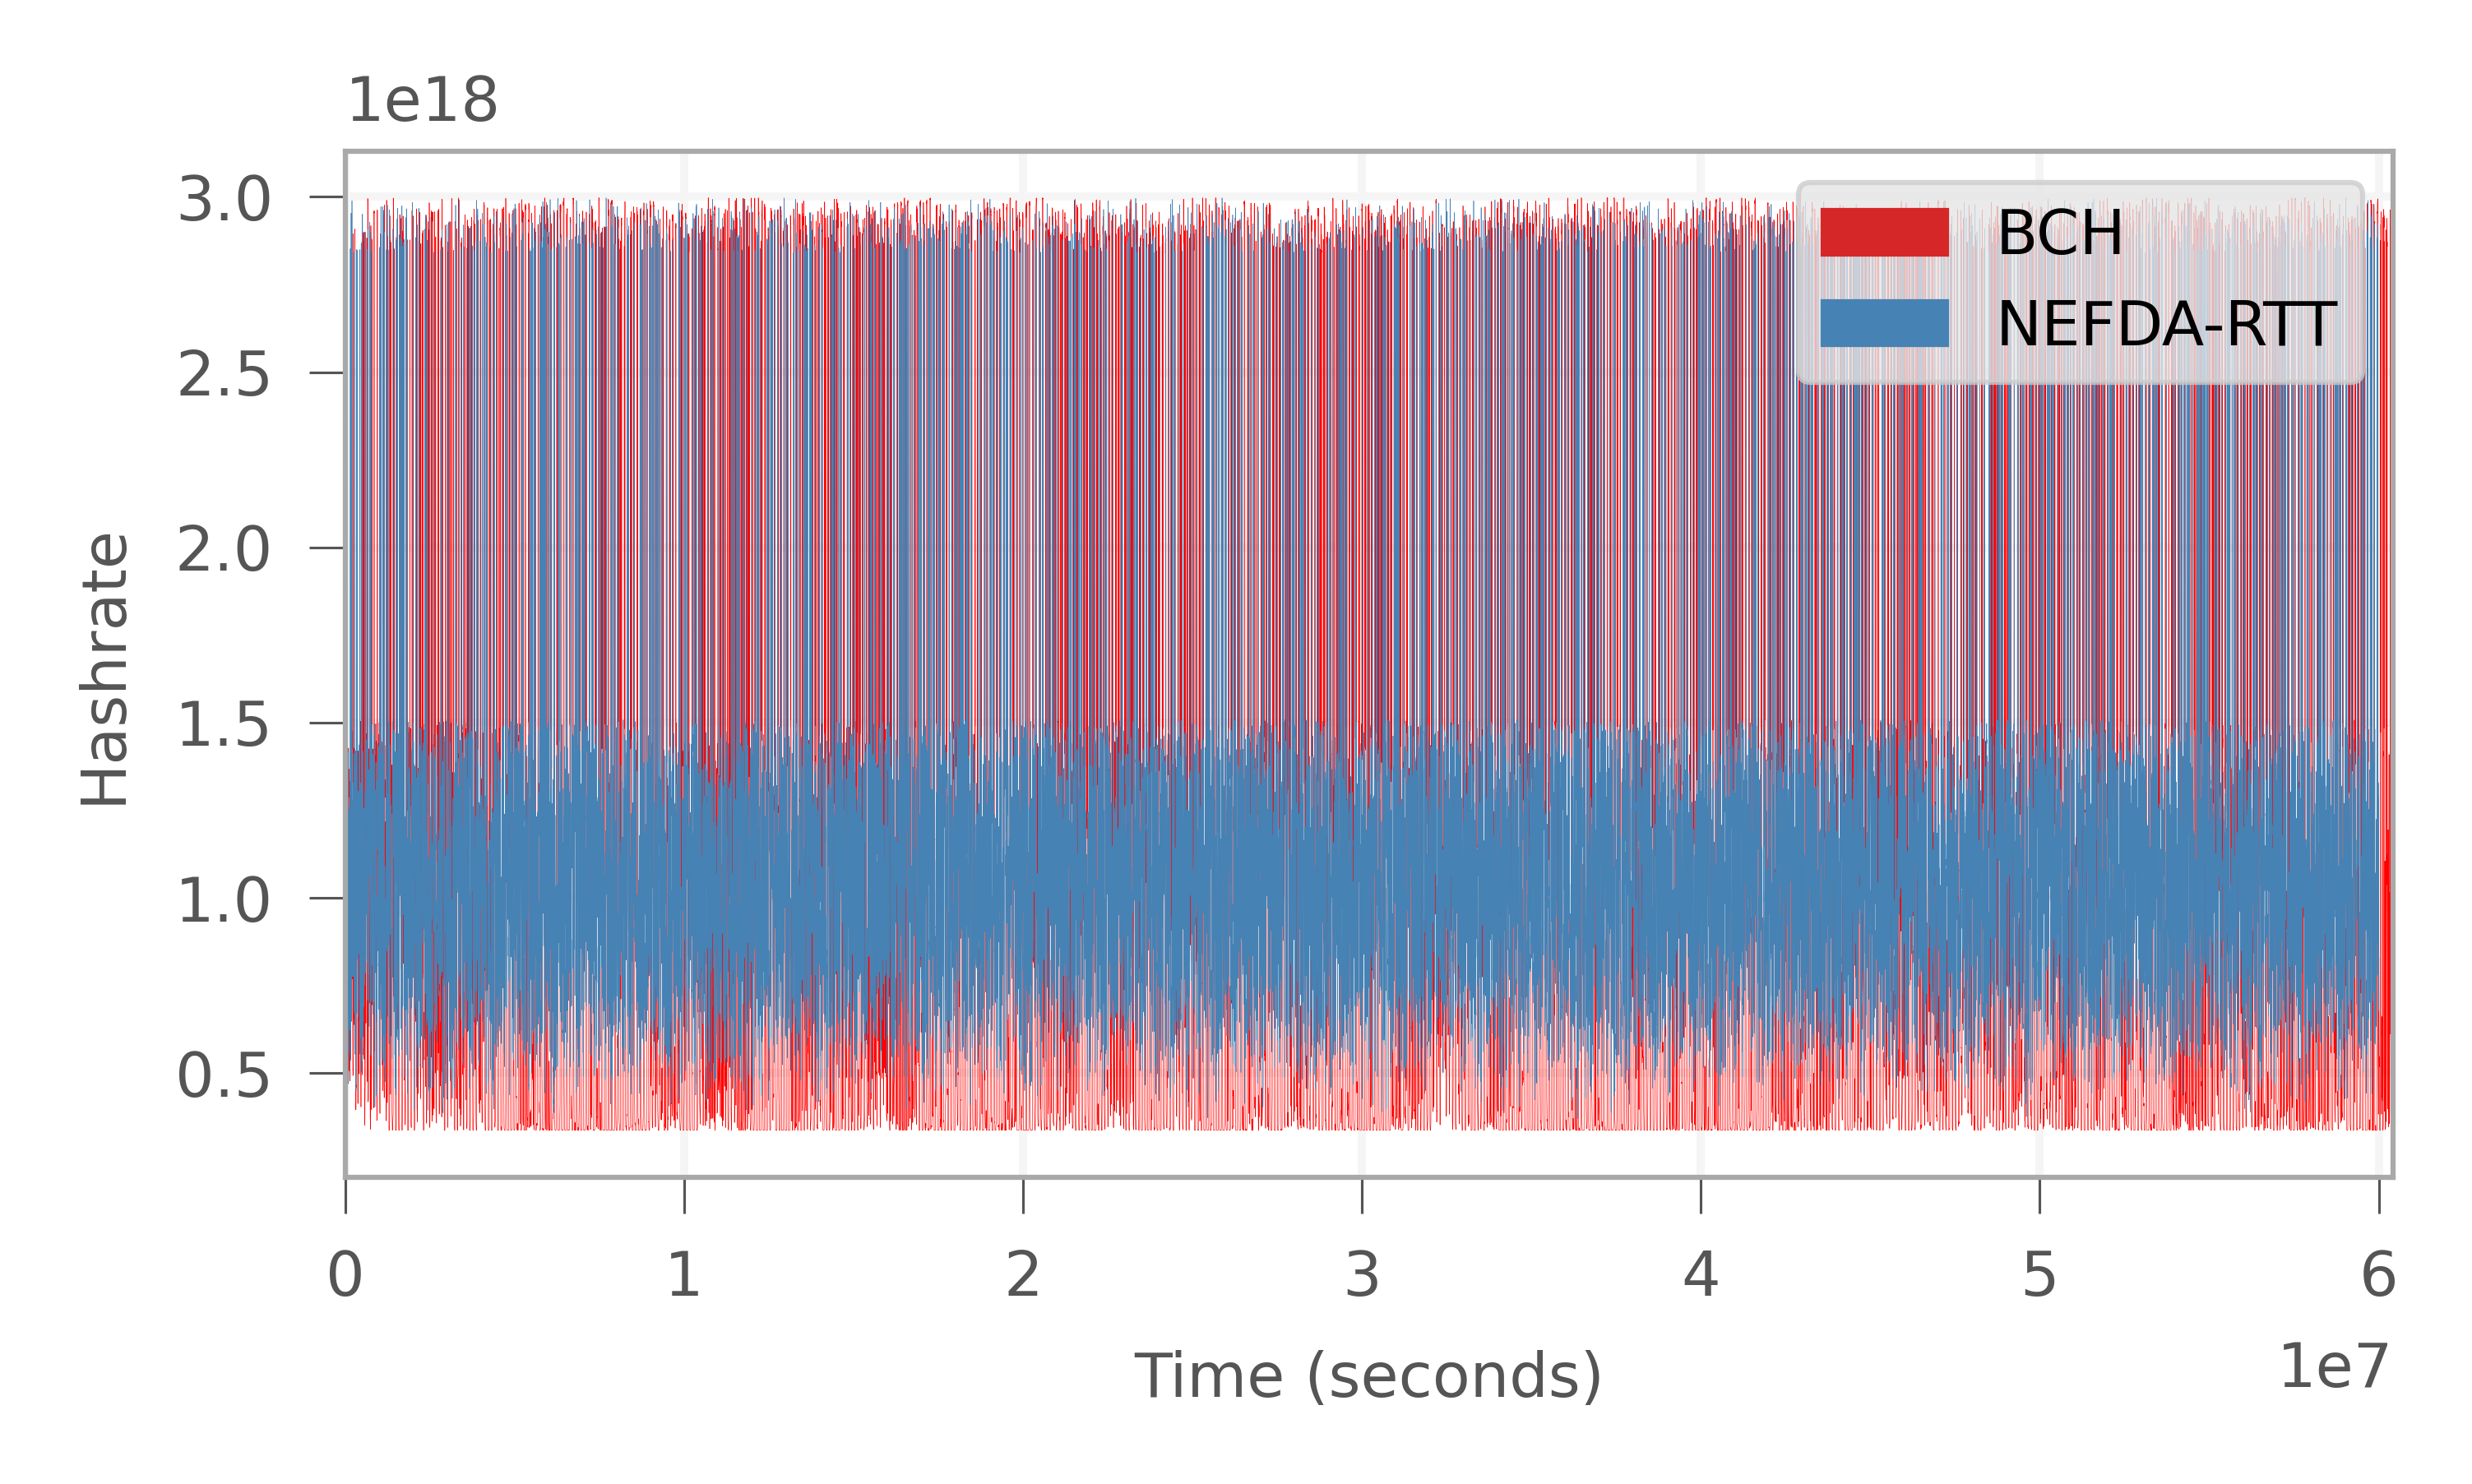}
\includegraphics[width=0.48\textwidth]{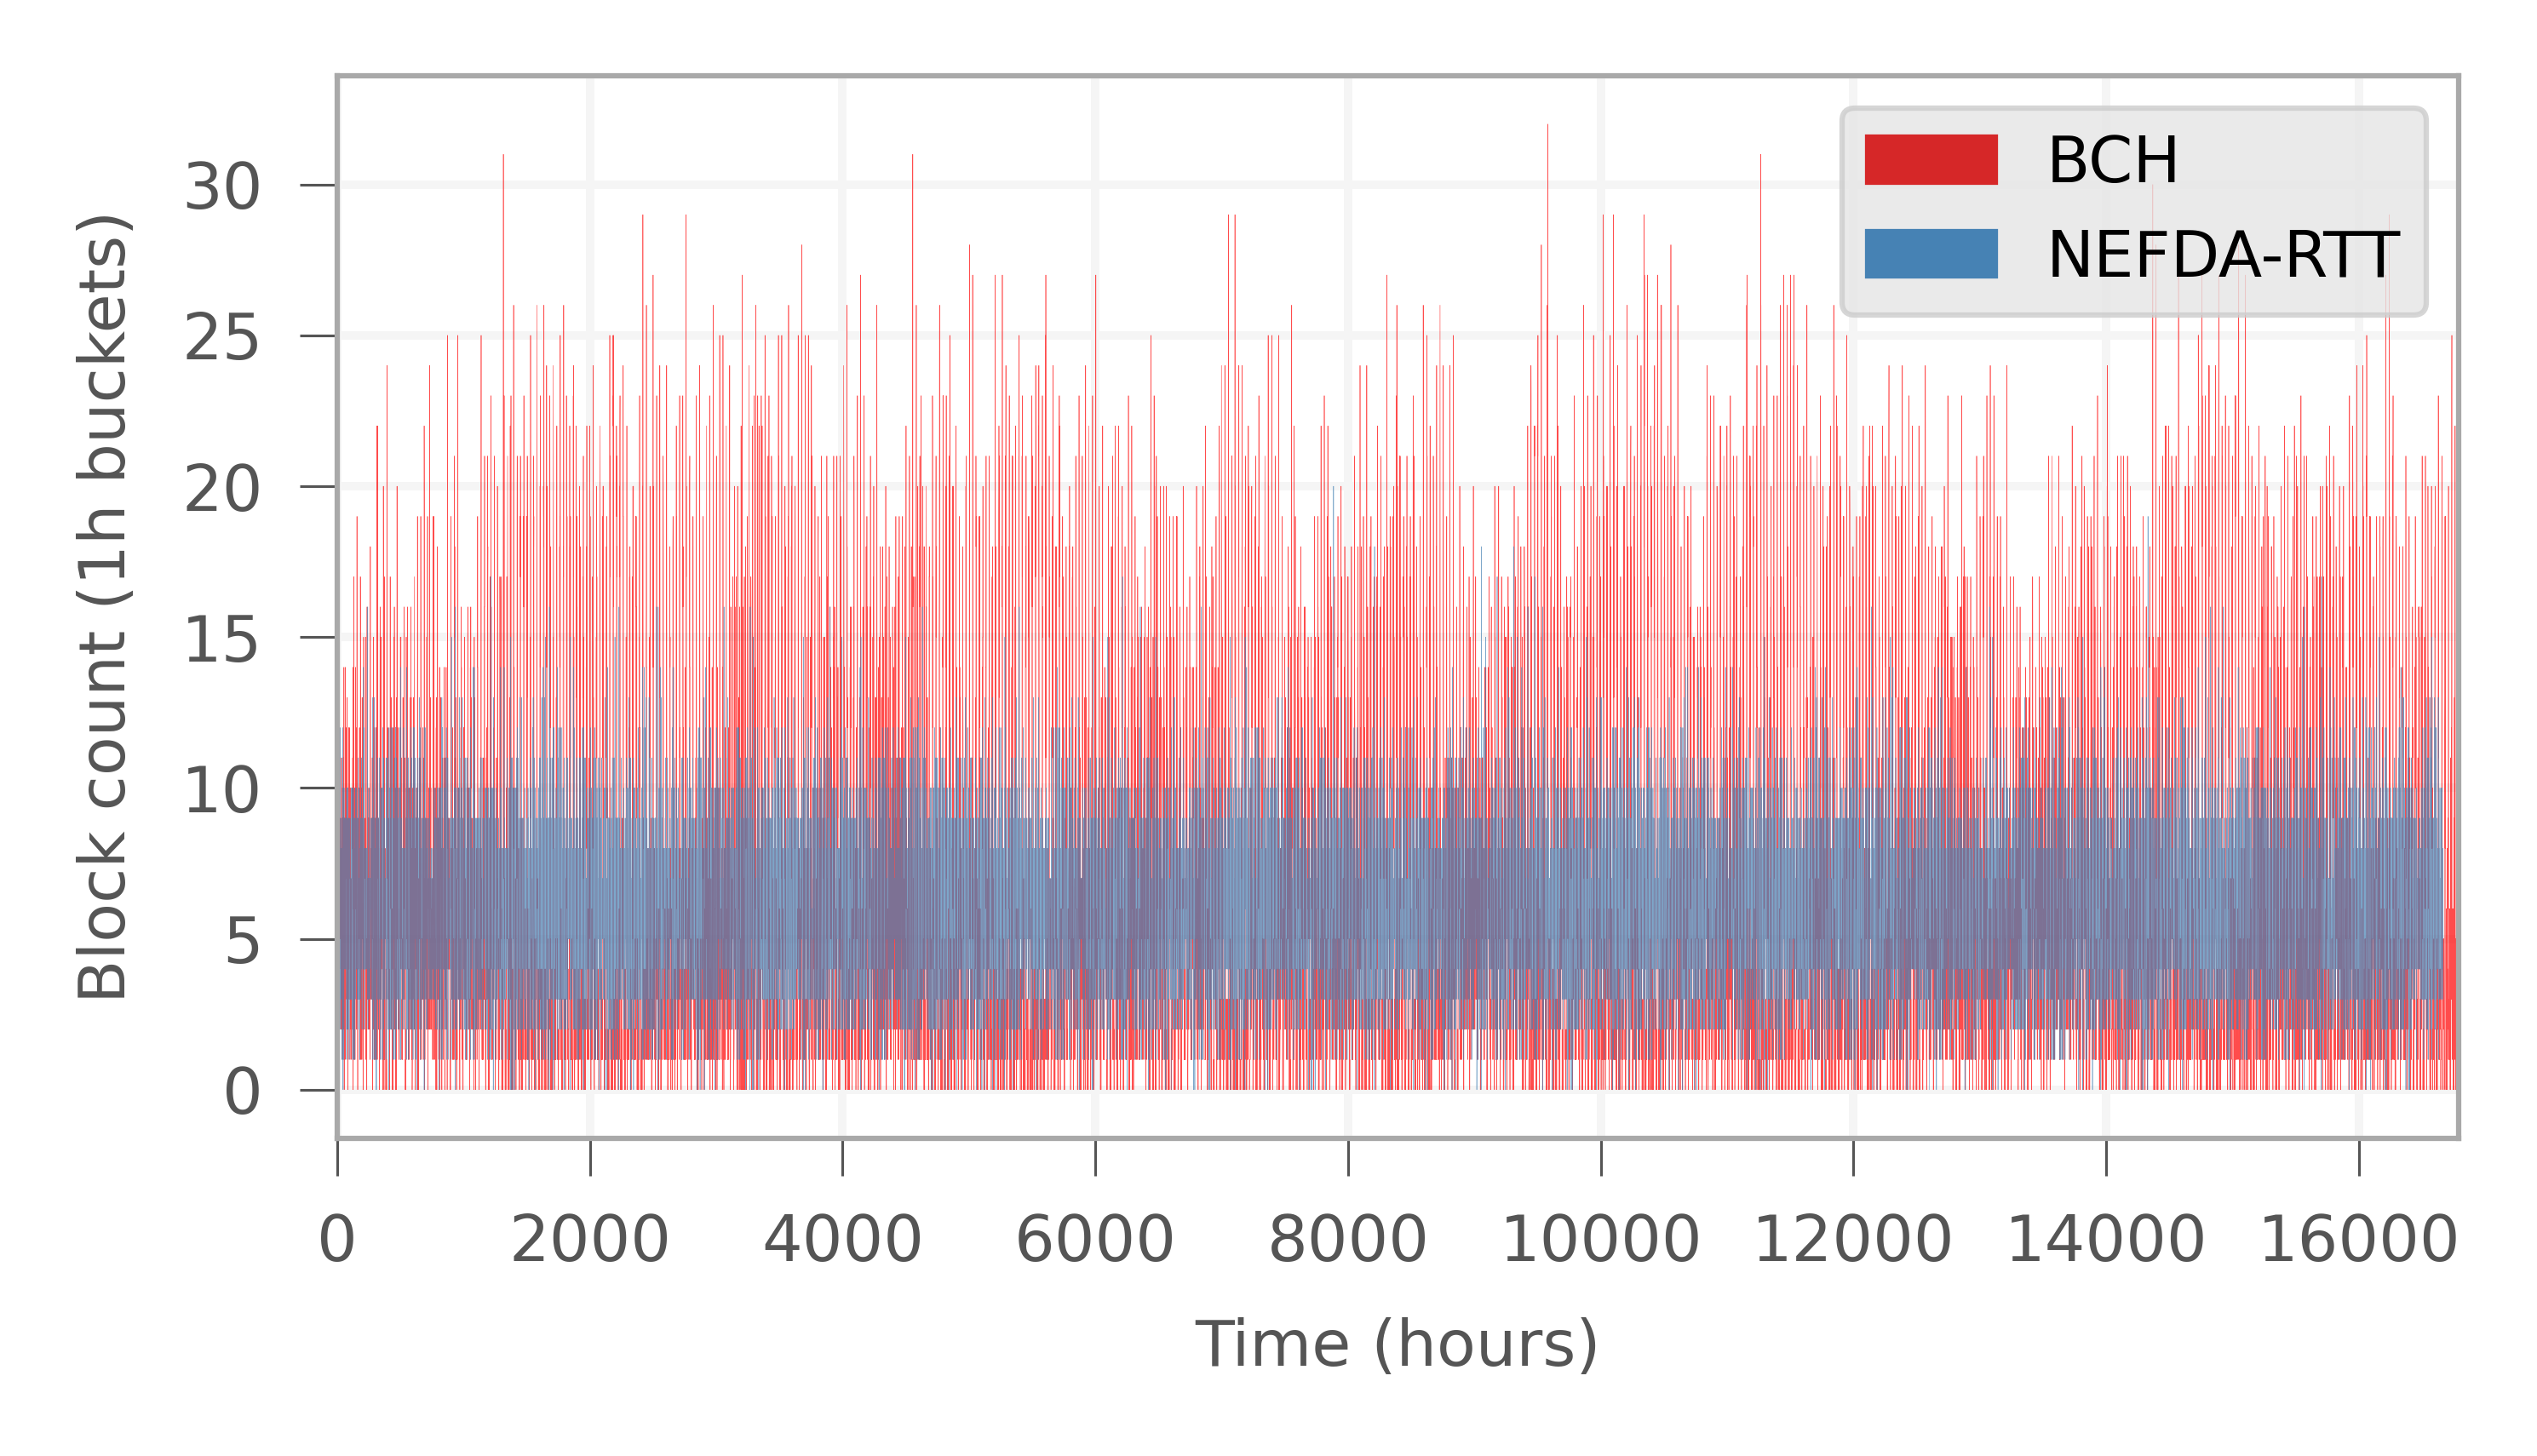}
\caption{The targets, hash rates and blocks mined per hour for NEFDA--RTT and Amaury's DA in a coin-hopping simulation of 100\,000 blocks.}
\label{sim:sigmoid-summary}
\end{figure}
